# Supplementary material for: Mind the Inconspicuous: Revealing the Hidden Weakness in Aligned LLMs' Refusal Boundaries
Source: arXiv:2405.20653 source file (2025-06-17)
Supplement: Supplementary file 1 [file broader.tex]

\section{Broader Impact}
\label{sec:braoder}
In this work, we propose a novel jailbreaking attack, \sys, that leverages the \eos token to jailbreak LLMs. This research can be used by malicious users to enhance their attacks on LLMs. Despite the potential risks, we believe it is important to disclose this vulnerability to the public. The strategy of \sys is straightforward and can be discovered by attackers independently. By disclosing this vulnerability, we can raise awareness of the potential risks of \eos tokens and encourage the community to develop effective defenses. We also provide recommendations for future research to mitigate the risks of \sys.

The positive impact of this work is to help the community have a better understanding of why LLMs can respond to harmful prompts even after red-teaming fine-tuning. Our work shows that the \major{refusal boundary} learned by LLMs is not robust and can be bypassed by simply appending \eos tokens. This finding can help researchers and practitioners better understand the limitations of existing red teaming fine-tuning and develop more robust defenses against harmful content generation.

\section{Ethical Considerations}
\label{sec:ethical}
Considering the potential risks of our work, we take the following measures to mitigate the negative impact of our research. First, we provide a content warning at the beginning of our paper to alert readers to the harmful language contained in our examples. Second, we notify the model providers of the potential risks of \sys prior to submission and provide recommendations for mitigating these risks. Third, we open-source the code and data used in our experiments to promote transparency and reproducibility. Finally, we provide recommendations for future research to mitigate the risks of \sys and encourage the community to develop effective defenses against this attack.

\section{Related Works}
\label{sec:related_works}
We summarize the related works in the following aspects.

\paragraph{Safety and Privacy of LLMs.}
Recent studies have revealed that LLMs are susceptible to various attacks, including jailbreak attacks~\cite{zou2023universal,yu2023gptfuzzer,deng2023jailbreaker}, prompt injection attacks~\cite{yu2023assessing,liu2023prompt}, and data poisoning attacks~\cite{shu2023exploitability,qiang2024learning}. These attacks target different vulnerabilities within LLMs, posing significant threats to their safety.

Jailbreak attacks exploit prompt engineering techniques to extract harmful information from LLMs. 
This harmful information can encompass hate speech, misinformation, or other detrimental content. 
Although the information produced by LLMs in these scenarios may not be directly actionable, responding to harmful prompts can increase the risk of real-world harm. 
For instance, \citet{zou2023universal} and \citet{yu2023gptfuzzer} have demonstrated white-box and black-box jailbreak strategies to bypass safety mechanisms in LLMs, leading to the generation of inappropriate content.

Prompt injection attacks, akin to injection attacks in software security, involve injecting malicious prompts to manipulate the generated text of LLMs. By leveraging prompt injection, attackers can influence the outputs of applications that integrate LLMs, such as judgment or decision-making systems. This manipulation is particularly concerning as it can lead to unwanted outcomes in real-world applications.
OWASP has recognized prompt injection as one of the top-10 threats to LLMs~\cite{owasp2024promptinjection}, underscoring the critical need to address this vulnerability. Prior work~\cite{yu2023assessing,liu2023prompt} has investigated the mechanics of prompt injection attacks and highlighted their potential impacts on the reliability of applications powered by LLMs.

Data poisoning attacks target the integrity of LLMs by contaminating their pre-training or fine-tuning datasets. Such attacks can subtly alter the behavior of LLMs, leading them to produce biased or malicious outputs. For example, \citet{shu2023exploitability} demonstrates that poisoning a small subset of fine-tuning data (e.g., 5\%) could compel an LLM to promote the attacker's product or excessively reject user requests. These studies highlight the necessity of understanding the security and privacy risks associated with LLMs and developing robust defenses to mitigate these threats.

As to the privacy of LLMs, recent works have shown that LLMs can memorize sensitive information from the training data~\cite{wang2023decodingtrust,zhang2024generated,sun2024trustllm,mattern2023membership} such as the email address or phone number of users. This memorization behavior poses a significant privacy risk to users, as it can lead to the inadvertent disclosure of sensitive information. By analyzing the generated text or output probability, the membership inference attack can infer whether a specific data point was present in the training data~\cite{mattern2023membership,zhang2024generated}. Those attacks pose great threats to the privacy of users and require effective defenses to mitigate the risks.

\paragraph{Defenses Against LLM Attacks.}
To mitigate the risks associated with various attacks on LLMs, numerous approaches have been proposed to ensure the alignment and security of these models across different stages. These approaches can be broadly categorized into defenses applied during the pre-training stage, fine-tuning stage, and inference stage.

During the pre-training stage, a critical defense mechanism involves filtering the training dataset to remove harmful or sensitive information. This preprocessing step aims to ensure that the LLM is not exposed to potentially malicious or sensitive information. For instance, prior work~\cite{welbl2021challenges} applies training set filters to remove explicit content from the training data.
These filters are designed to exclude explicit, biased, or otherwise harmful content, thereby reducing the likelihood that the LLM will generate such content in response to user prompts.

In the fine-tuning stage, developers can further enhance the model's safety by incorporating red-teaming examples~\cite{ganguli2022red, bai2022training, touvron2023llama,OpenAI2023GPT4TR,luo2024dapa}. This involves using carefully crafted adversarial prompts to train the LLM to recognize and refuse to generate harmful content. By exposing the model to a variety of malicious prompts during fine-tuning, developers can condition it to identify and reject harmful instructions, thereby improving its robustness against adversarial attacks. 

The inference stage, where the LLM interacts with end-users, can also be protected using various content filtering mechanisms. These filters operate in real-time to monitor and block the generation of harmful content. OpenAI’s moderation tools~\cite{openai2022moderation} and Perspective API~\cite{jigsaw2024perspectiveapi} train the classifier to detect harmful content. Similarly, researchers also find that LLM itself can be used to detect harmful content~\cite{lees2022new}.
These systems analyze the LLM's outputs and intervene when potentially harmful content is detected, ensuring that end-users are shielded from inappropriate or dangerous responses. By implementing these real-time filters, developers can add an additional layer of protection that dynamically responds to evolving threats.

By combining these defenses, the safety and privacy of LLMs can be enhanced, reducing the risks associated with various attacks.
