# Supplementary material for: Mind the Inconspicuous: Revealing the Hidden Weakness in Aligned LLMs' Refusal Boundaries
Source: arXiv:2405.20653 source file (2025-06-17)
Supplement: Supplementary file 2 [file appendix.tex]

% \part*{Supplementary Material}
% %\begin{center}
% %	{\LARGE \textbf{Appendix}}
% %\end{center}
% {
% \setlength{\parskip}{-0em}
% \startcontents[sections]
% \printcontents[sections]{ }{1}{}
% }

\section{\major{Refusal Boundary} Bypass}
\label{appendix:boundary}
\subsection{Dataset Construction}
\label{appendix:boundary_dataset}
\subsection{Visulization for Other Layers}
\label{appendix:vis}

\subsection{Varying the Number of \textit{eos} Tokens}
\label{appendix:vary}
\subsection{Shift Towards the Boundary}
\label{appendix:shift}

\section{Evaluation of Response}
\label{appendix:response}

\section{Additional Numerical Experiments}
\label{appendix:exp}
We further compare the GCG loss to analyze how \sys enhances the GCG attack. We plot the GCG loss of the original GCG and the GCG with \sys in \autoref{appendix:exp} on model Llama-2-chat-7B. From the figure, we can see that the initial GCG loss is lower and it decreases faster when \sys is integrated. This indicates that \sys can help the optimization process to find the adversarial suffix more efficiently.
