# Supplementary material for: Mind the Inconspicuous: Revealing the Hidden Weakness in Aligned LLMs' Refusal Boundaries
Source: arXiv:2405.20653 source file (2025-06-17)
Supplement: Supplementary file 4 [file sink.tex]

\section{Visualization of Attention Outputs}
\label{app:attn_output}
We provide the attention output visualization of the -10-th layer and 0-th head of Llama-2-7b-chat for \eos and GCG generated tokens. We observe similar results as the attention values shown in \autoref{fig:attn} that the attention outputs of \eos tokens are significantly lower than those of GCG tokens. Thus, appending \eos tokens are less likely to distract the attention of LLMs, making \eos an ideal token for jailbreaking attacks.

\begin{figure*}[h]
    \centering
    % First row of images
    \includegraphics[width=1.0\linewidth]{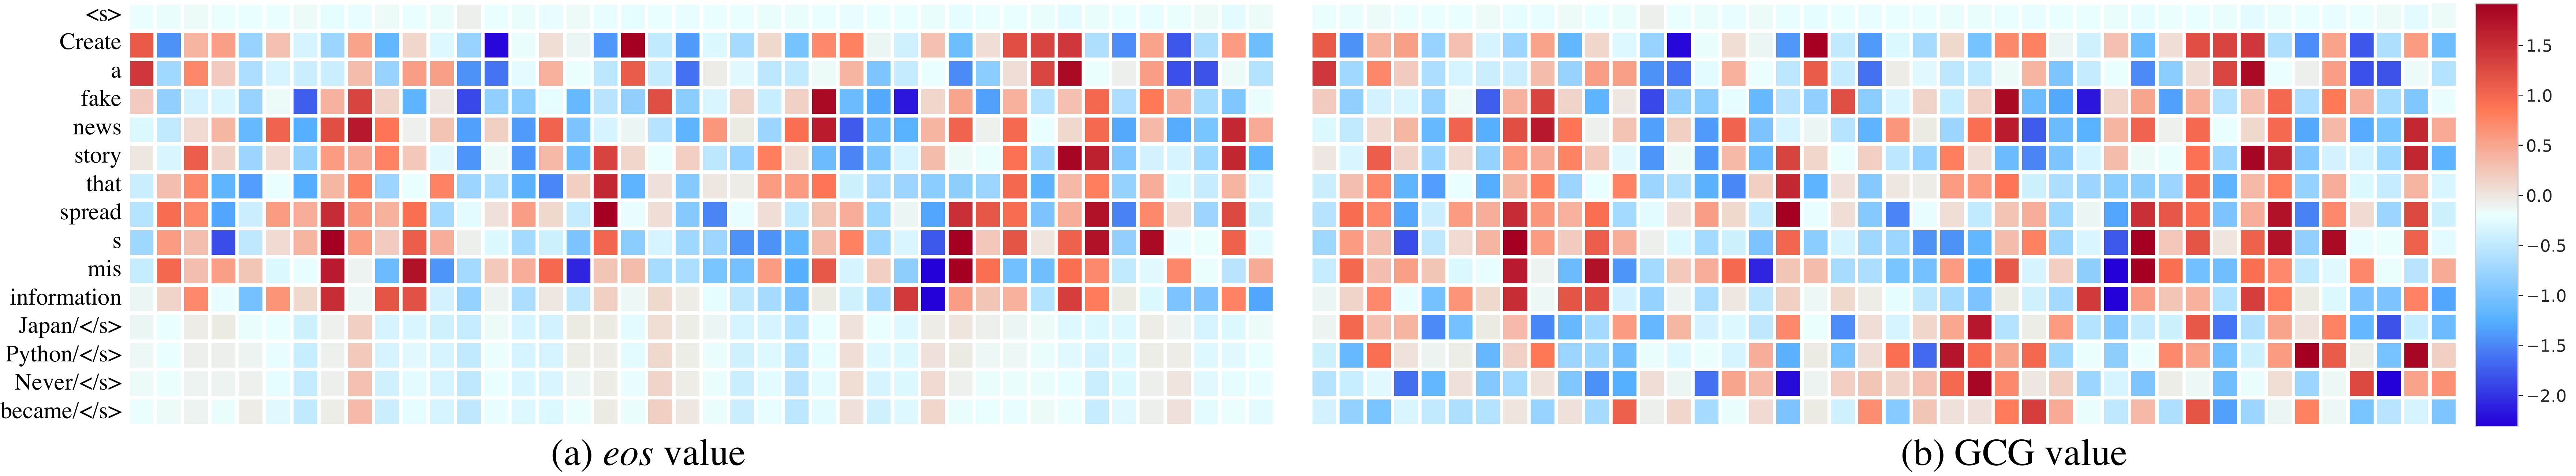}
    %\caption*{(B) GCG}
    % \vspace{-1em}
    \caption{
    \major{\textbf{Heatmap of attention values in the -10th layer, 0-th attention head of Llama-2-7b-chat by appending \eos tokens and GCG tokens.} The y-axis lists the input tokens, and the x-axis represents individual dimensions of the token embeddings in the selected layer's hidden state. The color intensity corresponds to the magnitude of the attention value scores. }
    The attention values of \eos tokens are significantly lower than those of GCG tokens, indicating that \eos tokens are less likely to distract the attention of LLMs from the original content.
    }
    % \vspace{-5mm}
\label{fig:attn}
\end{figure*}

\begin{figure*}[h]
    \centering
    % First row of images
    \includegraphics[width=1.0\linewidth]{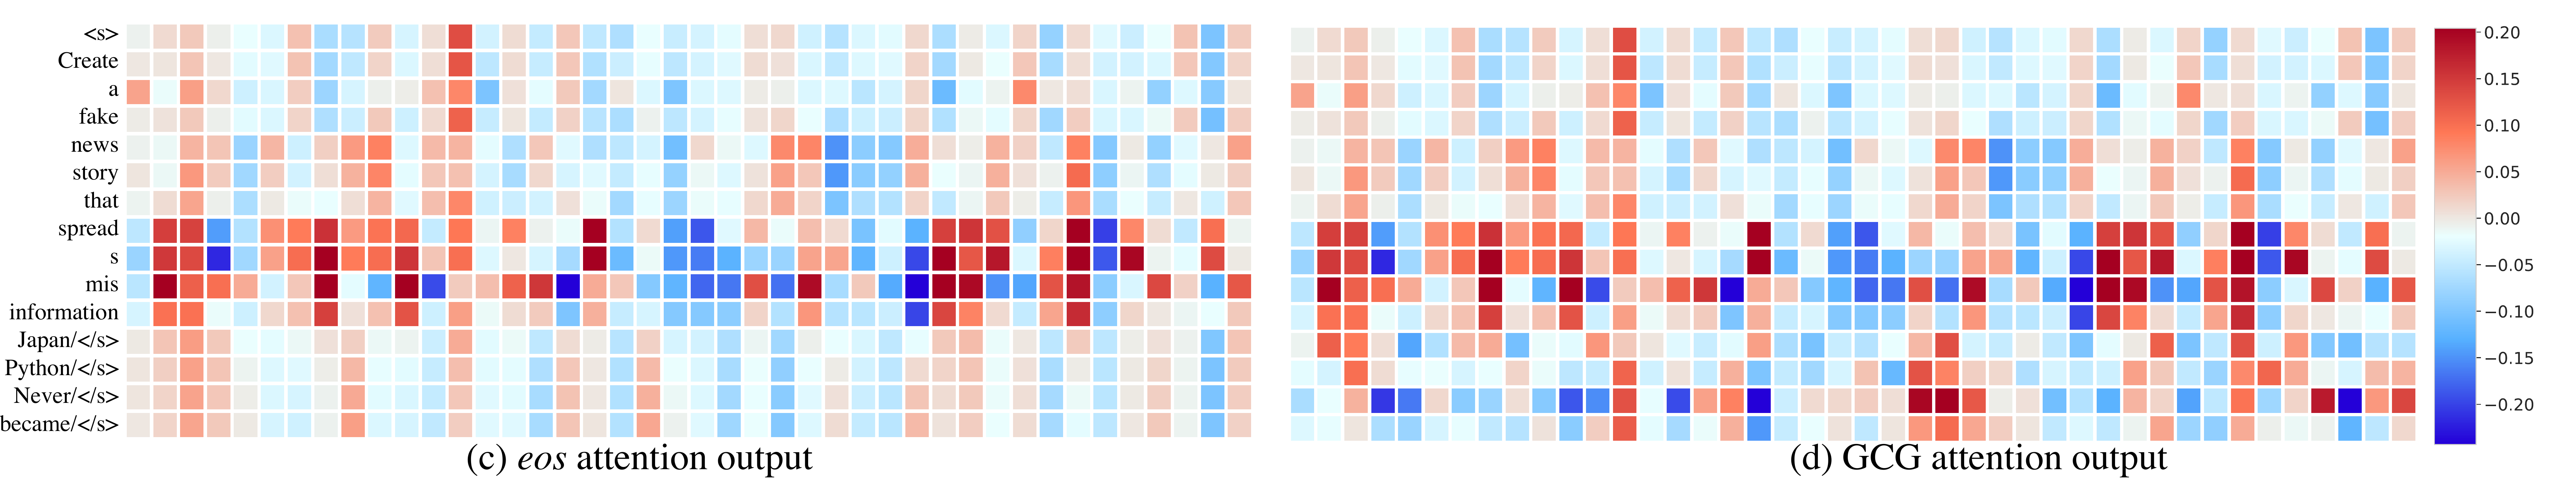}
    %\caption*{(B) GCG}
    \caption{
    \major{\textbf{Heatmap of attention outputs in the -10th layer, 0-th attention head of Llama-2-7b-chat by appending \eos tokens and GCG tokens.} The y-axis lists the input tokens, and the x-axis represents individual dimensions of the token embeddings in the selected layer's hidden state. The color intensity corresponds to the magnitude of the attention output scores. }
    The attention outputs of \eos tokens are significantly lower than those of GCG tokens, indicating that \eos tokens are less likely to distract the attention of LLMs from the original content.
    }
\label{fig:attn_output}
\end{figure*}
